# Supplementary material for: Narrow-linewidth homogeneous optical emitters in diamond nanostructures via silicon ion implantation
Source: arXiv:1512.03820 ancillary file (2016-04-25)
Supplement: Supplementary file 1 [file 1512.03820_SI.pdf]

# Supplementary Material for:
# Coherent optical emitters in diamond nanostructures via ion implantation

Ruffin E. Evans,[1,*] Alp Sipahigil,[1,*] Denis D. Sukachev,[1,2] Alexander S. Zibrov,[1] and Mikhail D. Lukin[1,†]

[1]*Department of Physics, Harvard University, 17 Oxford St., Cambridge, MA 02138*

[2]*Russian Quantum Center, Business-center "Ural", 100A Novaya St., Skolkovo, Moscow 143025*

**CONTENTS**

S1. Setup description 1

S2. Fabrication and implantation procedures 3
- A. Bulk SiV creation 3
- B. Nanofabrication 4

S3. Additional optical characterization 4
- A. Lifetime measurements and quantum yield 4
- B. Autocorrelation fluorescence measurements 5
- C. Saturation: linewidth as a function of power 5
- D. Inhomogeneous distribution of all transition frequencies 6

S4. Statistical methods 6

References 7

## S1. SETUP DESCRIPTION

The experiments were carried out in three different scanning confocal microscopes fabricated in-house. To perform the cryogenic measurements, we used two $4\,\mathrm{K}$ helium flow cryostats: a Janis Cryogenics model ST-500 and later a modified probe-station (Desert Cryogenics model TTP4). The room-temperature measurements of the bulk $\mathrm{SiV}^-$ centers used to extract the yield of the implantation process were performed in a separate room-temperature microscope. All three microscopes used a 0.95 NA microscope objective (Nikon CFI LU Plan Apo Epi 100×). In the cryogenic measurements, the objective was inside the vacuum chamber. A general schematic of the experimental apparatus is shown in Fig. S1.

Because the $\mathrm{SiV}^-$ linewidth is a strong function of the temperature[1], it is important to make sure the sample is as cold as possible. For our $\mathrm{SiV}^-$ linewidth measurements, we therefore place a thin indium foil spacer between the sample and the sample stage and clamp the sample to the indium and stage ($3.5\,\mathrm{K}$). Based on other measurements using this technique, we expect the temperature of the sample to be under about $6\,\mathrm{K}$. It is worth noting that in our experience other sample mounting techniques (silver paint, thermal grease, or varnish) have been less effective at reaching these low temperatures, primarily due to the radiation load from the room-temperature objective.

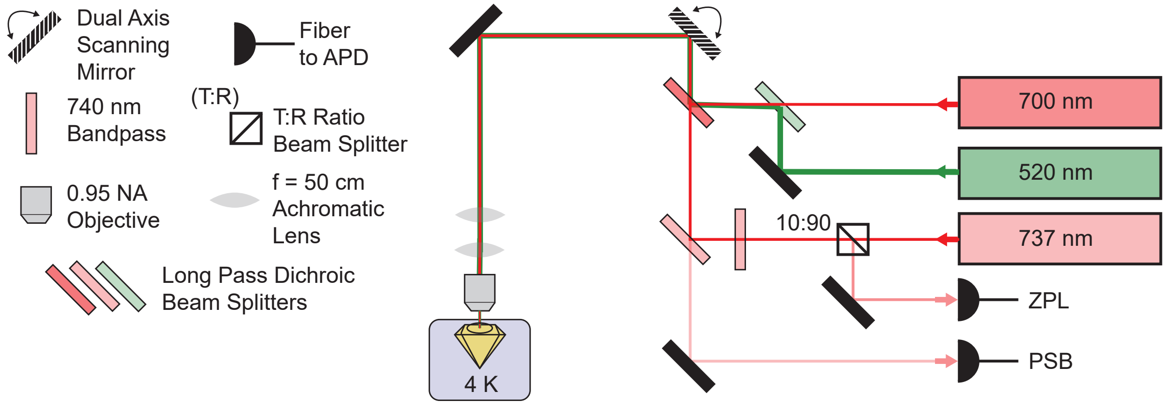


FIG. S1. General confocal microscope design. The 520 nm and 700 nm lasers are used to excite the $SiV^-$ off-resonantly. The 737 nm ECDL is used to excite the $SiV^-$ resonantly. Collection can be performed either on the ZPL (if the excitation is off-resonance) or the PSB (in either excitation scheme). For the cryogenic measurements, the objective and the sample are in the vacuum chamber and the sample is clamped to the cold finger of a flow-through cryostat.

To measure the fluorescence wavelengths of the $SiV^-$ centers (e.g. to produce the data in Fig. 1c and Fig. 2a, b) we excite the $SiV^-$ centers using off-resonant light (approximately 5 mW) from a 700 nm diode laser (Thorlabs LP705-SF15). Off-resonant excitation with a 520 nm diode laser (Thorlabs LP520-SF15) is also possible, and using both of these wavelengths together results in a superlinear enhancement in the observed count rate, suggesting that the 520 nm laser may play a role in stabilizing the $SiV^-$ charge state. The resulting fluorescence is sent to a spectrometer (Horiba iHR550 imaging spectrometer with Synapse CCD and $1800\,\mathrm{gr/mm}$) with a spectral resolution of $0.025\,\mathrm{nm}$. When describing the distribution of emitter wavelengths in Fig. 2 of the main text, transition C was always chosen for the samples annealed at 1100 °C. Although other transitions had slightly broader distributions, each transition had a much narrower distribution than after the 800 °C anneal (see Section S3 D). For the spectra taken after 800 °C annealing only, transition C was chosen whenever unambiguous assignment was possible. Occasionally, spectra had only one or two clear lines or contained broad features; in these cases, the brightest line (which should correspond to transition C) was chosen. Identifying the transitions after 1100 °C annealing was straightforward.

To measure the linewidths of the $SiV^-$ centers, we excite the $SiV^-$ center with a external-cavity diode laser (in Fig. 2D, based on Opnext Diode HL7302MG operated in the Littrow configuration; in Fig. 3, Newport/New Focus Velocity TLB-6711-P) resonant with the $SiV^-$ zero-phonon line (ZPL) around $406.62\,\mathrm{THz}$ (737 nm) and monitor the $SiV^-$ phonon-sideband (PSB) fluorescence. As we sweep over the $SiV^-$ resonance, we detect a peak in PSB counts. For all frequency scans, the instantaneous laser frequency is monitored and stabilized using a high resolution wavemeter (High Finesse WS7) with 10 MHz resolution and 50 MHz accuracy. This results in an approximately 25–50 MHz total laser linewidth over the course of the experiment. Single photons are detected using single photon counting modules (2 Picoquant $\tau$-SPADs and/or Excelitas SPCM-NIR, each with around 350 ps FWHM measured timing jitter). We use a laser noise eater (Thorlabs LCC3112H) to stabilize laser power to less than $1\%$ during frequency scans.

## S2. FABRICATION AND IMPLANTATION PROCEDURES

### A. Bulk SiV creation

We begin with an electronic-grade CVD diamond from Element Six Inc. The top surface has a $\{100\}$ crystallographic orientation. The concentrations of impurities are $[N]_S^0 < 5\,\mathrm{ppb}$ and $[B] < 1\,\mathrm{ppb}$. The sample is polished on a scaife by Element Six. After obtaining the sample, we perform an oxidative acid clean in $1:1:1$ conc. Nitric : conc. Sulfuric : 70% perchloric acid. The sample is placed in the acid mixture and boiled under reflux for at least 45 minutes, then allowed to cool and rinsed with ultrapure water (Millipore Direct-Q 3 or equivalent) and blow-dried out of isopropanol. This procedure is performed after each annealing step to remove graphitic carbon present on the diamond surface after annealing and also produces an oxygen surface termination[2–4].

The sample is then etched in a Unaxis Shuttleline inductively-coupled plasma reactive ion etcher (ICP RIE). This pre-fabrication etch ("pre-etch") reduces the surface roughness of the diamond sample and relieves strain created from the mechanical polishing process. The sample is first etched for 30 minutes with an $Ar/Cl_2$ plasma mixture to remove around two microns of diamond. This etch is followed by a 30-minute $O_2$ etch that removes around five microns of diamond. At the end of this process, the diamond surface has less than $1\,\mathrm{nm}$ RMS roughness over several square microns. More details on this technique can be found elsewhere[5, 6].

Next, we send the sample for implantation to Innovion corporation, where $^{29}\mathrm{Si}^+$ ions are implanted at $150\,\mathrm{keV}$ at a dose of $1 \times 10^{10}\,\mathrm{ions/cm^2}$. Based on calculations using the Stopping Range of Ions in Matter (SRIM) package[7], we predict that this energy should result in a Si depth of around $100\,\mathrm{nm}$ (Fig. S2).

After implantation, we perform high-temperature high-vacuum annealing. First, the chamber is heated over four hours to $400\,°\mathrm{C}$ to desorb water vapor from the chamber walls and lower the pressure inside the chamber. The temperature is held at $400\,°\mathrm{C}$ for eight hours, then ramped over twelve hours to $800\,°\mathrm{C}$. The primary purpose of this step is to create $\mathrm{SiV}^-$ centers through vacancy diffusion[8, 9]. The sample is then acid cleaned and characterized to determine the $\mathrm{SiV}^-$ yield and inhomogeneous distribution at this stage.

Next, the sample is annealed a second time. The steps up to $800\,°\mathrm{C}$ were identical to the previous anneal. After these steps, the temperature of the furnace is ramped over twelve hours to $1100\,°\mathrm{C}$. This slow ramp is necessary to keep the pressure in our furnace low ($\lesssim 10^{-6}\,\mathrm{Torr}$). This temperature is maintained for two hours. This step is designed to anneal out divacancies and other defects[10, 11]. As described in the main text, our microscopic understanding of the mechanisms behind these annealing steps is consistent with the observations that the yield does not increase after the $1100\,°\mathrm{C}$ anneal, but the inhomogeneous distribution becomes significantly lower. More details on this annealing procedure can be found elsewhere[6]. Before each annealing stage, we characterize the surface of the sample using X-ray photoelectron spectroscopy (Thermo Scientific K-Alpha XPS system) to verify that the surface is clean and free of contaminants (primarily Na, Cl, and Si). We did not perform a low-temperature anneal in an oxygen environment[6, 12]. The sample is again characterized to determine the $\mathrm{SiV}^-$ yield and inhomogeneous distribution. The procedure as outlined so far, with the exception of the pre-etch, was also repeated for a second sample.

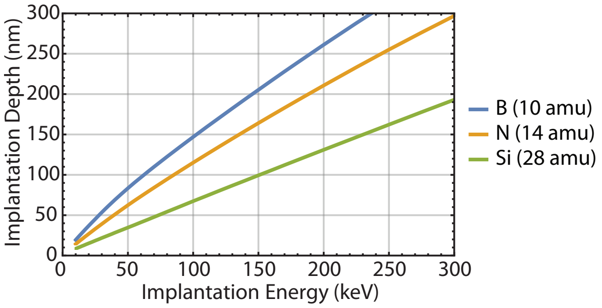


FIG. S2. Predicted depth as a function of implantation energy for a few common diamond dopants as calculated with the Stopping Range of Ions in Matter (SRIM) package. We use an implantation energy of 150 keV which should correspond to a depth of around 100 nm. This depth corresponds to an implantation energy of around 85 keV for nitrogen ions.

### B. Nanofabrication

After preparing and characterizing the bulk $\mathrm{SiV^-}$ centers as described above, we fabricate triangular diamond nanobeam waveguides in order to characterize the quality of the resulting $\mathrm{SiV^-}$ centers inside nanoscale photonic structures. A complete description of the properties and fabrication of these devices can be found elsewhere[5]. For completeness, and because our procedure differs slightly, we give a brief description of our nanofabrication procedure here.

First, we define a pattern using e-beam lithography (Elionix ELS-F125 lithography system, Microchem poly(methyl methacrylate) (PMMA) EL9/C2 resists). After development (1 : 3 methyl isobutyl ketone : isopropanol), we deposit approximately 200 nm of alumina using reactive sputtering of an aluminum target (AJA 3-target system) and then dissolve the PMMA in acetone to perform lift-off to define a mask. The chip is etched first top-down in a PlasmaTherm Versaline ICP RIE system in an oxygen plasma (170 V DC bias, 100 W RF bias, 700 W ICP power with 30 sccm $O_2$ flow rate at 10 mTorr chamber pressure) to define nanoscale posts. The chip is then placed in a macroscopic Faraday cage in the shape of a triangular prism and and etched with the same parameters to create free-standing triangular diamond nanobeams. Finally, the sample is acid cleaned, annealed using the 1100 °C recipe described above, and acid cleaned again.

## S3. ADDITIONAL OPTICAL CHARACTERIZATION

### A. Lifetime measurements and quantum yield

The consistent production of narrow linewidth $\mathrm{SiV^-}$ centers is a key result of this paper. In this context, "narrow" is relative to the lower bound on the linewidth determined by the lifetime. If the $\mathrm{SiV^-}$ has a radiatively limited lifetime, it is possible for the lifetime in nanostructures to be significantly longer since the effective refractive index is lower inside such a structure. To probe this effect, we measured the lifetime of nine $\mathrm{SiV^-}$ centers. The lifetime measured in the waveguides ($\tau = 1.69 \pm 0.14$ ns, N = 5) was not significantly different from the lifetime measured in the bulk-like anchors ($\tau = 1.75 \pm 0.08$ ns, N = 4). Both values are in good agreement with previously reported values in the literature[1, 12]. This implies that the lifetime of the $\mathrm{SiV^-}$ excited state is predominantly determined by a nonradiative decay rate. More thorough measurements of the $\mathrm{SiV^-}$ lifetime in different environments would

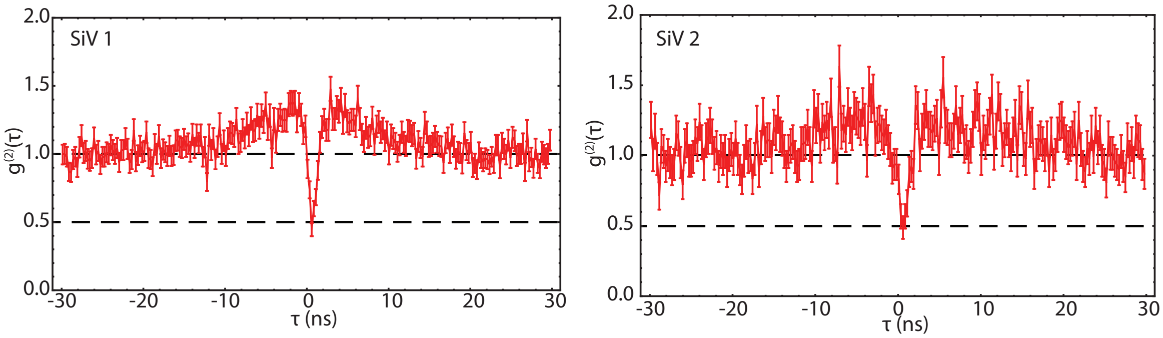


FIG. S3. Autocorrelation measurement of two $\mathrm{SiV}^-$ centers inside a diamond nanobeam as described in the text. Error bars are estimated assuming the noise on the number of detected photons follows a Poisson distribution (shot noise). The extent of the dip at $\tau = 0$ is limited by finite detector bandwidth.

be useful in determining the quantum yield exactly.

### B. Autocorrelation fluorescence measurements

To verify that the detected photons were emitted by single $\mathrm{SiV}^-$ centers, we performed fluorescence autocorrelation measurements on two $\mathrm{SiV}^-$ centers inside diamond nanobeams. We performed this measurement by exciting the $\mathrm{SiV}^-$ centers off resonantly as described above and splitting the emission between two detectors in a Hanbury-Brown–Twiss configuration. The relative arrival times of the photons on the two detectors were recorded using fast acquisition electronics (PicoQuant HydraHarp 400) with a resolution better than $128\,\mathrm{ps}$. The data were binned into $256\,\mathrm{ps}$ intervals.

The relative photon detection times $g^{(2)}(\tau)$ (normalized by defining $g^{(2)}(\infty) = 1$) are displayed in Fig. S3. For a single quantum emitter, the signal at zero time delay should have $g^{(2)}(0) = 0$. A value of $g^{(2)}(0) < 0.5$ would confirm that we are measuring emitters producing single photons. Our data show a dip of $g^{(2)}(0) \sim 0.5$. However, finite jitter on our detectors (Section S1) of around $350\,\mathrm{ps}$ causes the measured arrival times of our photons to be convolved with the detector response, hence limiting the sharpness and minimum value of our dip. This explains why our autocorrelation measurements do not show the full dip expected for a single quantum emitter[13].

### C. Saturation: linewidth as a function of power

To assure that our linewidths were not limited by power broadening, we measured the linewidth of an $\mathrm{SiV}^-$ center as a function of applied laser power $I$ (Fig. S4). To check qualitative agreement of this data with theory, we fit these linewidth based on the expected response of a two-level system: $\Delta\nu(I) = A\sqrt{1 + BI}$ with fit parameters $A$ and $B$. The agreement is quite good and the value at zero power is consistent with the (low-power) linewidths reported in the main text. The error bars on the data are the standard error in the fit parameters estimated from the variance in the data.

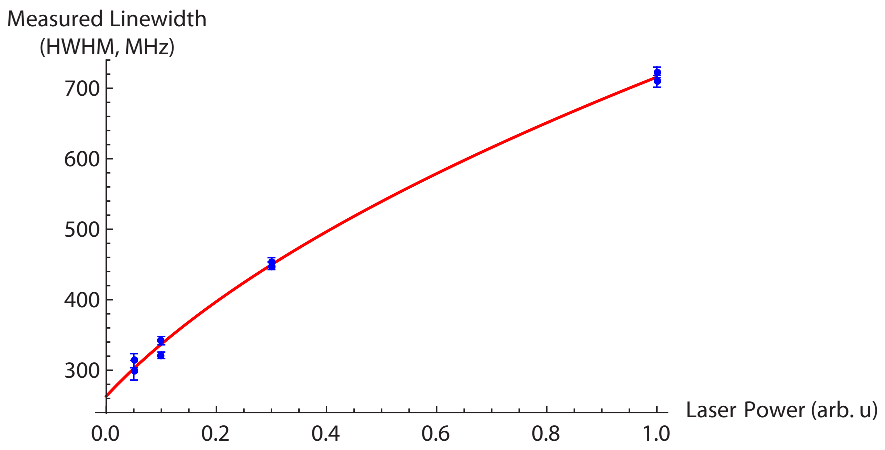


FIG. S4. Measurement of an $\mathrm{SiV}^-$ linewidth as a function of applied laser power. The data (blue points) are fit to the functional dependence expected for a two-level system (red line) as described in the text.

### D. Inhomogeneous distribution of all transition frequencies

In the main text (e.g. Fig. 2), we focused on the optical transition frequencies of transition C and noted the reduction in inhomogeneous distribution after $1100\,°\mathrm{C}$ annealing relative to $800\,°\mathrm{C}$ annealing. This reduction in inhomogeneous distribution is also present for the other optical transitions of the $\mathrm{SiV}^-$ center. In Fig. 2c, we plot a composite spectrum constructed by summing over all of the 13 spectra taken from different $\mathrm{SiV}^-$ centers after $1100\,°\mathrm{C}$ annealing. To account for spectrum-to-spectrum intensity variations, each spectrum is normalized (after subtracting a constant background) and contributes equally to the sum. This composite spectrum is very similar to the spectrum of a single unstrained $\mathrm{SiV}^-$ center (Fig. 1c) and shows the expected fine-structure splitting. This demonstrates that the inhomogeneous distribution of $\mathrm{SiV}^-$ transition wavelengths is generally small compared to the fine-structure splitting. For example, the effective "linewidth" of transition C in this composite spectrum is about the same as the inhomogeneous distribution reported in the main text. (The disagreement in these quantities is due to the finite resolution of the spectrometer.) The increased intensity to the red of the main peaks at $737\,\mathrm{nm}$ arises from summing over several transition D peaks from highly strained emitters that appear in this wavelength range. The corresponding transition A peaks expected to the blue of the main peaks are probably suppressed by a combination of unfavorable branching ratios and phonon-induced decay of the upper excited state during the excited state lifetime[1].

## S4. STATISTICAL METHODS

Because the distributions in Fig. 2a of the main text have very different widths, we represent these distributions with kernel density estimations (KDEs). Also, KDEs generally give a better overall representation of the underlying distribution than histograms do. The bandwith of the Gaussian kernel is set by the normal dis-

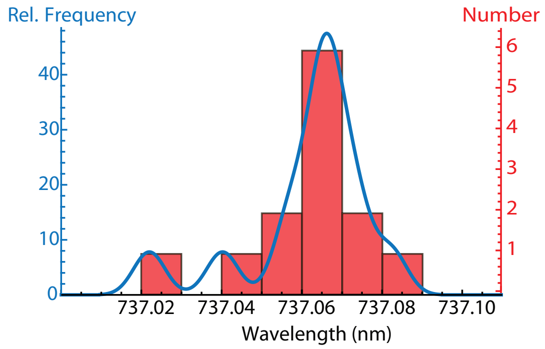


FIG. S5. Distribution of $SiV^-$ transition C wavelengths after annealing at 1100 °C. The data are represented both as a kernel density estimation (blue curve) and a histogram (red boxes). The kernel density estimation is the same as that shown in Fig. 2 of the main text.

tribution approximation (Silverman's rule). We use the kernel density estimation features implemented by the `SmoothKernelDistribution` and `SmoothHistogram` functions of Mathematica. A comparison of the kernel density estimation for transition C to histograms of the same data is shown in Fig. S5. The kernel density estimation for transition C closely follows the shape of the histogram.

---

* These authors contributed equally.
† lukin@physics.harvard.edu

[1] K. D. Jahnke, A. Sipahigil, J. M. Binder, M. W. Doherty, M. Metsch, L. J. Rogers, N. B. Manson, M. D. Lukin, and F. Jelezko, New J. Phys. **17**, 043011 (2015).
[2] U. D'Haenens-Johansson, A. Edmonds, B. Green, M. Newton, G. Davies, P. Martineau, R. Khan, and D. Twitchen, Phys. Rev. B **84**, 245208 (2011).
[3] M. Hauf, B. Grotz, B. Naydenov, M. Dankerl, S. Pezzagna, J. Meijer, F. Jelezko, J. Wrachtrup, M. Stutzmann, F. Reinhard, *et al.*, Phys. Rev. B **83**, 081304 (2011).
[4] A. Gali and J. R. Maze, Phys. Rev. B **88**, 235205 (2013).
[5] M. J. Burek, N. P. de Leon, B. J. Shields, B. J. Hausmann, Y. Chu, Q. Quan, A. S. Zibrov, H. Park, M. D. Lukin, and M. Loncar, Nano Lett. **12**, 6084 (2012).
[6] Y. Chu, N. de Leon, B. Shields, B. J. Hausmann, R. Evans, E. Togan, M. J. Burek, M. Markham, A. Stacey, A. Zibrov, *et al.*, Nano Lett. (2014).
[7] J. F. Ziegler, M. D. Ziegler, and J. P. Biersack, Nuclear Instruments and Methods in Physics Research Section B: Beam Interactions with Materials and Atoms **268**, 1818 (2010).
[8] G. Davies, S. C. Lawson, A. T. Collins, A. Mainwood, and S. J. Sharp, Phys. Rev. B **46**, 13157 (1992).
[9] P. Deák, B. Aradi, M. Kaviani, T. Frauenheim, and A. Gali, Phys. Rev. B **89**, 075203 (2014).
[10] V. Acosta, E. Bauch, M. Ledbetter, C. Santori, K.-M. Fu, P. Barclay, R. Beausoleil, H. Linget, J. Roch, F. Treussart, *et al.*, Phys. Rev. B **80**, 115202 (2009).
[11] T. Yamamoto, T. Umeda, K. Watanabe, S. Onoda, M. Markham, D. Twitchen, B. Naydenov, L. McGuinness, T. Teraji, S. Koizumi, *et al.*, Phys. Rev. B **88**, 075206 (2013).
[12] B. Pingault, J. N. Becker, C. H. Schulte, C. Arend, C. Hepp, T. Godde, A. I. Tartakovskii, M. Markham, C. Becher, and M. Atatüre, Phys. Rev. Lett. **113**, 263601 (2014).
[13] A. Sipahigil, K. D. Jahnke, L. J. Rogers, T. Teraji, J. Isoya, A. S. Zibrov, F. Jelezko, and M. D. Lukin, Phys. Rev. Lett. **113**, 113602 (2014).
